# Supplementary material for: Stochastic Continuous Submodular Maximization: Boosting via Non-oblivious Function
Source: arXiv:2201.00703 source file (2022-06-10)
Supplement: Supplementary file 1 [file Appendix-C.tex]

\noindent In this section, we verify the Theorem 4. First, we prove the following Lemma,
\begin{lemma}\label{lemma:c1} If we set the $\tilde{\nabla}_{B} F(\boldsymbol{x}_t)=\frac{1-e^{-\gamma}}{B\gamma}\sum_{i=1}^{B}\tilde{\nabla}f(z_{t,i}*\boldsymbol{x}_{t})$, for any $\mu_{t}>0$ and $\boldsymbol{x}^{*}\in\mathcal{C}$, we have
\begin{align*}
    F(\boldsymbol{x}_{t+1})-F(\boldsymbol{x}_{t})&\ge\eta((1-e^{-\gamma})f(\boldsymbol{x}^{*})-f(\boldsymbol{x}_{t}))-\eta_{t}(\frac{1}{\mu_{t}}\left\|\boldsymbol{s}_{t+1}-\boldsymbol{x}^{*}\right\|_{2}^{2}+\mu_{t}\left\|\nabla F(\boldsymbol{x}_{t})-\tilde{\nabla}_{B} F(\boldsymbol{x}_t) \right\|_{2}^{2})-\frac{L_{\gamma}}{2}\eta^{2}\left\|\boldsymbol{s}_{t+1}-\boldsymbol{x}_{t}\right\|_{2}^{2}
\end{align*}
\end{lemma}
\begin{proof}
\begin{equation} \label{equ:54}
    \begin{aligned}
    &F(\boldsymbol{x}_{t+1})-F(\boldsymbol{x}_{t})\\
    &=\int_{0}^{1}\langle \boldsymbol{x}_{t+1}-\boldsymbol{x}_{t}, \nabla F(\boldsymbol{x}_{t}+z(\boldsymbol{x}_{t+1}-\boldsymbol{x}_{t}))\rangle dz \\
    &\ge \langle \boldsymbol{x}_{t+1}-\boldsymbol{x}_{t}, \nabla F(\boldsymbol{x}_t) \rangle-\frac{L_{\gamma}}{2}\left\|\boldsymbol{x}_{t+1}-\boldsymbol{x}_{t}\right\|_{2}^{2}\\
    &=\eta\langle \boldsymbol{s}_{t+1}-\boldsymbol{x}_{t}, \nabla F(\boldsymbol{x}_t) \rangle-\frac{L_{\gamma}}{2}\eta^{2}\left\|\boldsymbol{s}_{t+1}-\boldsymbol{x}_{t}\right\|_{2}^{2}\\
    &=\eta(\langle \boldsymbol{s}_{t+1}-\boldsymbol{x}_{t}, \tilde{\nabla}_{B} F(\boldsymbol{x}_t)\rangle+\langle \boldsymbol{s}_{t+1}-\boldsymbol{x}_{t}, \nabla F(\boldsymbol{x}_{t})-\tilde{\nabla}_{B} F(\boldsymbol{x}_t) \rangle)-\frac{L_{\gamma}}{2}\eta^{2}\left\|\boldsymbol{s}_{t+1}-\boldsymbol{x}_{t}\right\|_{2}^{2}\\
    &\ge\eta(\langle \boldsymbol{x}^{*}-\boldsymbol{x}_{t}, \tilde{\nabla}_{B} F(\boldsymbol{x}_t) \rangle+\langle \boldsymbol{s}_{t+1}-\boldsymbol{x}_{t}, \nabla F(\boldsymbol{x}_{t})-\tilde{\nabla}_{B} F(\boldsymbol{x}_t) \rangle)-\frac{L_{\gamma}}{2}\eta^{2}\left\|\boldsymbol{s}_{t+1}-\boldsymbol{x}_{t}\right\|_{2}^{2}\\
    &=\eta(\langle \boldsymbol{x}^{*}-\boldsymbol{x}_{t}, \nabla F(\boldsymbol{x}_t) \rangle+\langle \boldsymbol{s}_{t+1}-\boldsymbol{x}^{*}, \nabla F(\boldsymbol{x}_{t})-\tilde{\nabla}_{B} F(\boldsymbol{x}_t)) \rangle)-\frac{L_{\gamma}}{2}\eta^{2}\left\|\boldsymbol{s}_{t+1}-\boldsymbol{x}_{t}\right\|_{2}^{2}\\
    &\ge\eta((1-e^{-\gamma})f(\boldsymbol{x}^{*})-f(\boldsymbol{x}_{t}))-\eta(\frac{1}{\mu_{t}}\left\|\boldsymbol{s}_{t+1}-\boldsymbol{x}^{*}\right\|_{2}^{2}+\mu_{t}\left\|\nabla F(\boldsymbol{x}_{t})-\tilde{\nabla}_{B} F(\boldsymbol{x}_t) \right\|_{2}^{2})\\&-\frac{L_{\gamma}}{2}\eta^{2}\left\|\boldsymbol{s}_{t+1}-\boldsymbol{x}_{t}\right\|_{2}^{2},
    \end{aligned}
\end{equation} where the first inequality follows that $F$ is $L_{\gamma}$-$smooth$ property of $F$ where $L_{\gamma}=L\frac{\gamma+e^{-\gamma}-1}{\gamma^{2}}$; the second from the definition of $\boldsymbol{s}_{t+1}$; the final from Young's inequality( for any $\mu_{t}>0$) and $\langle \boldsymbol{x}^{*}-\boldsymbol{x}_{t}, \nabla F(\boldsymbol{x}_t) \rangle\ge(1-e^{-\gamma})f(\boldsymbol{x}^{*})-f(\boldsymbol{x}_{t+1})$.
\end{proof}
With the ~\cref{lemma:c1}, we prove the Theorem 4.
\begin{proof}
\noindent From the ~\cref{lemma:c1}, we have
\begin{equation}\label{equ:55}
    \begin{aligned}
    &\mathbb{E}(\sum_{t=1}^{T-1}f(\boldsymbol{x}_{t})+\frac{F(\boldsymbol{x}_{T})}{\eta})\\
    &\ge(1-e^{-\gamma})(T-1)f(\boldsymbol{x}^{*})-\sum_{t=1}^{T}(\mathbb{E}(\eta(\frac{1}{\mu_{t}}\left\|\boldsymbol{s}_{t+1}-\boldsymbol{x}^{*}\right\|^{2}+\mu_{t}\left\|\nabla F(\boldsymbol{x}_{t})-\tilde{\nabla}_{B}F(\boldsymbol{x}_{t}) \right\|^{2})+\frac{L_{\gamma}}{2}\eta^{2}\left\|\boldsymbol{s}_{t+1}-\boldsymbol{x}_{t}\right\|^{2}))\\
    &\ge(1-e^{-\gamma})(T-1)f(\boldsymbol{x}^{*})-\sum_{t=1}^{T}(\mathbb{E}(\frac{1}{\mu_{t}}\mathrm{diam}^{2}(\mathcal{C})+\mu_{t}\frac{\sigma^{2}_{\gamma}}{B}+\frac{L_{\gamma}}{2}\eta\mathrm{diam}^{2}(\mathcal{C}))),
    \end{aligned}
\end{equation} where the second inequality follows from 
$\E(\left\|\nabla F(\boldsymbol{x}_{t})-\tilde{\nabla}_{B}F(\boldsymbol{x}_{t}) \right\|^{2})\le\frac{\sigma_{\gamma}^{2}}{B}$, $\left\|\boldsymbol{s}_{t+1}-\boldsymbol{x}^{*}\right\|\le\mathrm{diam}(\mathcal{C})$ and $\left\|\boldsymbol{s}_{t+1}-\boldsymbol{x}_{t}\right\|\le\mathrm{diam}(\mathcal{C})$.
 
If we set $\mu_{t}=\frac{\sqrt{B}\mathrm{diam}(\mathcal{C})}{\sigma_{\gamma}}$ in~\cref{equ:55}, we have
\begin{equation}\label{equ:c1}
    \begin{aligned}
    &\E(\sum_{t=1}^{T-1}f(\boldsymbol{x}_{t})+\frac{1+\ln(\tau)}{\eta}(f(\boldsymbol{x}_{T})+c))\\&\ge\E(\sum_{t=1}^{T-1}f(\boldsymbol{x}_{t})+\frac{F(\boldsymbol{x}_{t})}{\eta})\\&\ge(1-e^{-\gamma})(T-1)f(\boldsymbol{x}^{*})-\frac{T\mathrm{diam}(\mathcal{C})\sigma_{\gamma}}{\sqrt{B}}-\frac{L_{\gamma}\mathrm{diam}^{2}(\mathcal{C})\eta T}{2},
    \end{aligned}
\end{equation} where the first inequality follows from the Theorem 2; the second inequality comes from that we set $\mu_{t}=\frac{\sqrt{B}\mathrm{diam}(\mathcal{C})}{\sigma_{\gamma}}$ in~\cref{equ:55}.

According to the definition of $\triangle_{t}$ and $\triangle$ in Algorithm 3, we have $\triangle=\sum_{t=1}^{T}\triangle_{t}=T-1+\frac{1+\ln(\tau)}{\eta}$. Thus, we have

\begin{equation}\label{equ:56}
     \begin{aligned}
        \mathbb{E}(\sum_{t=1}^{T}\frac{\triangle_{t}}{\triangle}f(\boldsymbol{x}_{t}))&\ge(1-e^{-\gamma})\frac{\sum_{t=1}^{T}\triangle_{t}}{\triangle}f(\boldsymbol{x}^{*})-\frac{O(\frac{T}{\sqrt{B}})+O(\eta T)+O(\frac{1}{\eta})}{T-1+(1+\ln(\tau))/\eta}\\
        &\ge(1-e^{-\gamma}-\frac{(1+\ln(\tau))/\eta}{T-1+(1+\ln(\tau))/\eta})f(\boldsymbol{x}^{*})-\frac{\sum_{t=1}^{T}\triangle_{t}}{\triangle}f(\boldsymbol{x}^{*})-\frac{O(\frac{T}{\sqrt{B}})+O(\eta T)+O(\frac{1}{\eta})}{T-1+(1+\ln(\tau))/\eta}\\
        &\ge(1-e^{-\gamma}-O(\frac{1}{\sqrt{T}}))f(\boldsymbol{x}^{*})-O(\frac{1}{\sqrt{T}}),
     \end{aligned}
 \end{equation} where the final equality follows that we set $c=O(1)$, $B=O(T)$ and $\eta=O(1/\sqrt{T})$.
 \end{proof}
 Therefore, the Algorithm 3 returns a solution with $(1-e^{-\gamma}-\epsilon)\mathrm{OPT}-\epsilon$ after
