# Supplementary material for: Stochastic Continuous Submodular Maximization: Boosting via Non-oblivious Function
Source: arXiv:2201.00703 source file (2022-06-10)
Supplement: Supplementary file 2 [file Appendix-E.tex]

Recently, the \citet{mitra2021submodular+} investigate the continuous DR-submodular maximization with concave regularization, in which they take a similar non-oblivious method (Algorithm (4) in \citet{mitra2021submodular+}) to improve the Gradient Combining Frank-Wolfe algorithm (Algorithm (3) in \citet{mitra2021submodular+}). As a result, the Non-oblivious Frank-Wolfe (Algorithm (4) in \citet{mitra2021submodular+}) boosts the approximation ratio of submodular part from $(1/2)$ to $(1-1/e)$. In this section, we demonstrate some relationships between our devised non-oblivious function $F(\boldsymbol{x})$ and that of \cite{mitra2021submodular+}. In \cite{mitra2021submodular+}, they propose an auxiliary function $G(\boldsymbol{x})$ for DR-submodular function $f(\boldsymbol{x})$, i.e., for fixed $\epsilon$, 
\begin{equation}\label{equ:31}
   \begin{aligned}
        G(\boldsymbol{x})=\sum_{j=1}^{\epsilon^{-1}}\frac{e^{\epsilon j}f(\epsilon j*\boldsymbol{x})}{j}.
    \end{aligned}
\end{equation}
We observe that $\nabla G(\boldsymbol{x})=\epsilon\sum_{j=1}^{\epsilon^{-1}}e^{\epsilon j}\nabla f(\epsilon j*\boldsymbol{x})$. Also, if assuming $\nabla f(z*\boldsymbol{x})$ is integrable w.r.t. $z\in[0,1]$, for any fixed $\boldsymbol{x}$, we have $\lim_{\epsilon\rightarrow 0}G(\boldsymbol{x})=\int_{z=0}^{1}e^{z}\nabla f(z*\boldsymbol{x})dz=e\nabla F(\boldsymbol{x})$ when $\gamma=1$. Naturally, we could view the $\nabla G(\boldsymbol{x})$ as a discrete approximation to our proposed $\nabla F(\boldsymbol{x})$, since we are not surprised with the theoretical improvement of this function $G$. However, in \citep{mitra2021submodular+}, they do not give the motivation why they design the auxiliary function $G(\boldsymbol{x})$ in that form. In contrast, we derive the non-oblivious function $F(x)$ via the factor-revealing optimization equation~\eqref{equ:19} for improving the performance of stationary points. As a result, the non-oblivious function $F$ we propose could boost these existed optimization algorithms converging to stationary points, besides the classical Frank-Wolfe\citep{mitra2021submodular+,lacoste2016convergence}, from (1/2)-approximation to (1-1/e)-approximation.
Also, from Theorem (1), we also know the function $F$ satisfying $\nabla F(\boldsymbol{x})=\int_{z=0}^{1}e^{\gamma(z-1)}\nabla f(z*\boldsymbol{x})\mathrm{d}z$ is optimal in some sense.
